# Supplementary material for: Optimal Drive-by Sensing in Urban Road Networks with Large-scale Ridesourcing Vehicles
Source: arXiv:2207.11285 source file (2023-08-22)
Supplement: Supplementary file 1 [file 0_appendix.tex]

\newpage
\appendix
\section{Proof of proposition~\ref{prop:equivalent_condition}}~\label{appdix:proof_prop1}
\textbf{Proposition~\ref{prop:equivalent_condition}}
\textit{Suppose $\mathbf{R}^{\star}$ is the optimal solution to the maximization of $H^{t}$ in Eq.~\eqref{eq:entropy_of_IG}), then $\mathbf{R}^{\star}$ is also the optimal solution to the maximization of the sensing power in Eq.~\eqref{eq:veh_based_sensing_power}.} % prop1:equivalent

\begin{proof}
Without loss of generality, we formulate the objective in Eq.~\eqref{eq:entropy_of_IG} as a maximum entropy problem under the constraint $\sum\limits_{(i,j)\in \mathcal{A}}P_{ij}^{t}=1, \forall t \in \mathcal{T}$, since both problems have the same feasible region. For simplicity, we express $P_{ij}$ in replace of $P_{ij}^{t},t \in\mathcal{T}$ in the following proof. We solve the constrained optimization using Lagrangian relaxation with multiplier $\lambda$, which can be expressed as:
\begin{equation}
    \mathcal{L}\left(P_{i,j},\lambda\right) = -\sum_{(i,j)\in \mathcal{A}} P_{ij}\log P_{ij}+\lambda \left(1-\sum_{(i,j)\in \mathcal{A}} P_{ij}\right)
    \label{eq:lagrangian}
\end{equation}
Then we have the partial derivatives as below:
\begin{align}
        \frac{\partial\mathcal{L}}{\partial P_{ij}}&= -\log{P_{ij}}-1-\lambda\\
        \frac{\partial\mathcal{L}}{\partial\lambda}&= - \left(1-\sum\limits_{(i,j)\in \mathcal{A}} P_{ij}\right)
\end{align}

Following the first-order necessary condition, let the partial derivatives $\frac{\partial\mathcal{L}}{\partial P_{ij}}=0$ and $\frac{\partial\mathcal{L}}{\partial\lambda}=0$. Then we have:
\begin{equation}
    P_{ij} =\frac{1}{|\mathcal{A}|}= \exp{\left(-1-\lambda\right)}~\label{eq:optimality_sol}
\end{equation}
Hence, the maximum entropy is achieved when $P_{ij}$ follows the uniform distribution. 

We will next show that the same condition holds for maximizing the sensing power in Eq.~\eqref{eq:veh_based_sensing_power}, where the sensing frequency $P_{ij}=\frac{1}{|\mathcal{A}|},(i,j)\in\mathcal{A}$. Given each component $P_{ij}$ are non-negative, we can reformulate it following the geometric-mean inequality, which takes the form:
\begin{align}
    1-\frac{1}{|\mathcal{A}|} \sum_{(i,j)\in \mathcal{A}}\left(1-P_{ij}\right)^{|\mathcal{R}^{t}|}
    &\le 1-\left(\prod_{(i,j)\in\mathcal{A}}\left(1-P_{ij}\right)^{|\mathcal{R}^{t}|}\right)^{\frac{1}{|\mathcal{A}|}}~\label{eq:geometry_mean_ineq}\\
    &= 1-\left(\prod_{(i,j)\in\mathcal{A}}\left(1-P_{ij}\right)\right)^{\frac{|\mathcal{R}^{t}|}{|\mathcal{A}|}}
\end{align}
where the equality in Eq.~\eqref{eq:geometry_mean_ineq} holds if and only if each component $\left(1-P_{ij}\right)$ is equal~\citep{abramowitz1988handbook}. Recalling that $P_{ij}$ is the sensing frequency and $\sum\limits_{(i,j)\in\mathcal{A}}P_{ij}=1$, we therefore have $P_{ij}=\frac{1}{|\mathcal{A}|}$, which indicates the same optimal solution in Eq.~\eqref{eq:optimality_sol}.
\end{proof}

\section{Detailed results}

\subsection{Results for other time periods in Figure~\ref{fig:veh_sensing_points}}

\begin{figure}[H]
    \centering
    \includegraphics[width = 0.9\linewidth]{fig/filtered_traffic_by_interval_2.pdf}
    \caption{Spatial distribution of the RV visit frequency (on a log scale of 10). The circled region indicates the hot spots near Turtle Bay.}
\end{figure}

% \subsection{Results for other time periods in Figure~\ref{fig:fleet_info_coverag_weekday}}

% \begin{figure}
%      \centering
%         \includegraphics[width=0.9\textwidth]{fig/spatial_temporal_inferred_info_day20_2.pdf}
%          \caption{Spatial distribution of observations on a weekday using inferred information (U: unknown, I: inferred, O: observed.)}\label{appendix_fig:spatial_distribution_link_ob}
% \end{figure}

\subsection{Detailed results for Algorithm~\ref{algo:solution_algo} in other time periods}

\begin{table}[H]
    \centering
    \scriptsize
    \caption{{Results of the K-shortest Path-based algorithm and comparison with historical trajectory}}
    \label{appendix_tab:rerouting_performance_comparison}
    \begin{tabular}{c|c|c|c|c|c|c|c|c|c|c|c}
    \toprule
    $t$                       & Scenario               &$\delta$ & $K$& $c^{exp}$& $c^{inf}$ & $c^{imp}$ &  $H^{t}$  & $S^{t}$ & $\Delta D$& $\Delta T$ & CPU\_Time\\\hline
  12 PM - 3 PM &  before &    - &  - &  0.76 &   0.98 &     0.98 &     6.59 &          0.63 &               0.00 &                0.00 &        - \\
 12 PM - 3 PM &   after &    0.9 &  20 &  0.88 &   0.99 &     0.98 &     6.84 &          0.78 &              11.02 &                7.62 &  80.2265 \\
 12 PM - 3 PM &   after &    0.9 &  40 &  0.88 &   0.99 &     0.98 &     6.85 &          0.78 &              16.85 &                9.86 &  157.308 \\
 12 PM - 3 PM &   after &    0.9 &  60 &  0.89 &   0.99 &     0.99 &     6.86 &          0.78 &              19.34 &               10.81 &  235.039 \\
 12 PM - 3 PM &   after &    0.9 &  80 &  0.89 &   0.99 &     0.99 &     6.86 &          0.78 &              21.40 &               11.60 &  311.446 \\
 12 PM - 3 PM &   after &    1.0 &  20 &  0.89 &   0.99 &     0.99 &     6.86 &          0.78 &              18.13 &               10.35 &  87.2639 \\
 12 PM - 3 PM &   after &    1.0 &  40 &  0.89 &   0.99 &     0.99 &     6.87 &          0.79 &              24.31 &               12.72 &  170.216 \\
 12 PM - 3 PM &   after &    1.0 &  60 &  0.89 &   0.99 &     0.99 &     6.88 &          0.79 &              27.12 &               13.80 &  255.065 \\
 12 PM - 3 PM &   after &    1.0 &  80 &  0.89 &   0.99 &     0.99 &     6.88 &          0.79 &              29.93 &               14.88 &  334.361 \\
 12 PM - 3 PM &   after &    1.1 &  20 &  0.89 &   0.99 &     0.99 &     6.88 &          0.79 &              27.06 &               13.78 &  94.8827 \\
 12 PM - 3 PM &   after &    1.1 &  40 &  0.90 &   0.99 &     0.99 &     6.89 &          0.80 &              33.94 &               16.41 &  187.568 \\
 12 PM - 3 PM &   after &    1.1 &  60 &  0.90 &   0.99 &     0.99 &     6.90 &          0.80 &              37.71 &               17.86 &  275.977 \\
 12 PM - 3 PM &   after &    1.1 &  80 &  0.90 &   0.99 &     0.99 &     6.90 &          0.80 &              40.63 &               18.98 &  363.788 \\
 12 PM - 3 PM &   after &    1.2 &  20 &  0.90 &   0.99 &     0.99 &     6.89 &          0.79 &              33.42 &               16.22 &   101.53 \\
 12 PM - 3 PM &   after &    1.2 &  40 &  0.90 &   0.99 &     0.99 &     6.91 &          0.80 &              40.27 &               18.84 &  200.396 \\
 12 PM - 3 PM &   after &    1.2 &  60 &  0.90 &   0.99 &     0.99 &     6.92 &          0.81 &              44.86 &               20.61 &  301.035 \\
 12 PM - 3 PM &   after &    1.2 &  80 &  0.90 &   0.99 &     0.99 &     6.92 &          0.81 &              48.50 &               22.00 &  399.697 \\\hline
    6 PM - 9 PM &  before &    - &  - &  0.76 &   0.97 &     0.98 &     6.56 &          0.62 &               0.00 &                0.00 &        - \\
  6 PM - 9 PM &   after &    0.9 &  20 &  0.86 &   0.98 &     0.98 &     6.79 &          0.75 &              10.24 &                7.47 &  81.7234 \\
  6 PM - 9 PM &   after &    0.9 &  40 &  0.87 &   0.98 &     0.98 &     6.81 &          0.76 &              16.75 &                9.75 &  160.135 \\
  6 PM - 9 PM &   after &    0.9 &  60 &  0.87 &   0.98 &     0.98 &     6.82 &          0.76 &              20.44 &               11.03 &  241.639 \\
  6 PM - 9 PM &   after &    0.9 &  80 &  0.87 &   0.99 &     0.98 &     6.82 &          0.76 &              22.45 &               11.74 &  321.342 \\
  6 PM - 9 PM &   after &    1.0 &  20 &  0.87 &   0.99 &     0.98 &     6.80 &          0.76 &              16.23 &                9.56 &  87.8938 \\
  6 PM - 9 PM &   after &    1.0 &  40 &  0.87 &   0.99 &     0.98 &     6.82 &          0.76 &              23.25 &               12.02 &  172.902 \\
  6 PM - 9 PM &   after &    1.0 &  60 &  0.88 &   0.99 &     0.98 &     6.83 &          0.77 &              26.99 &               13.32 &  256.728 \\
  6 PM - 9 PM &   after &    1.0 &  80 &  0.88 &   0.99 &     0.98 &     6.84 &          0.77 &              30.22 &               14.45 &  343.103 \\
  6 PM - 9 PM &   after &    1.1 &  20 &  0.88 &   0.99 &     0.98 &     6.81 &          0.76 &              20.46 &               11.04 &  91.6479 \\
  6 PM - 9 PM &   after &    1.1 &  40 &  0.88 &   0.99 &     0.98 &     6.83 &          0.77 &              28.40 &               13.82 &  184.082 \\
  6 PM - 9 PM &   after &    1.1 &  60 &  0.88 &   0.99 &     0.98 &     6.84 &          0.77 &              32.43 &               15.23 &   274.42 \\
  6 PM - 9 PM &   after &    1.1 &  80 &  0.88 &   0.99 &     0.98 &     6.84 &          0.77 &              35.77 &               16.39 &  364.028 \\
  6 PM - 9 PM &   after &    1.2 &  20 &  0.88 &   0.99 &     0.98 &     6.82 &          0.76 &              27.38 &               13.46 &  95.9781 \\
  6 PM - 9 PM &   after &    1.2 &  40 &  0.88 &   0.99 &     0.98 &     6.84 &          0.77 &              36.68 &               16.71 &  195.263 \\
  6 PM - 9 PM &   after &    1.2 &  60 &  0.88 &   0.99 &     0.98 &     6.85 &          0.77 &              41.67 &               18.45 &  297.134 \\
  6 PM - 9 PM &   after &    1.2 &  80 &  0.89 &   0.99 &     0.98 &     6.86 &          0.77 &              45.31 &               19.73 &  392.449 \\ \hline
 12 AM - 3 AM &  before &    - &  - &  0.77 &   0.98 &     0.98 &     6.59 &          0.67 &               0.00 &                0.00 &        - \\
 12 AM - 3 AM &   after &    0.9 &  20 &  0.88 &   0.99 &     0.99 &     6.85 &          0.81 &               1.62 &                4.86 &  78.8375 \\
 12 AM - 3 AM &   after &    0.9 &  40 &  0.89 &   0.99 &     0.99 &     6.87 &          0.82 &               6.10 &                6.70 &  156.135 \\
 12 AM - 3 AM &   after &    0.9 &  60 &  0.89 &   0.99 &     0.99 &     6.88 &          0.82 &               8.48 &                7.67 &  235.338 \\
 12 AM - 3 AM &   after &    0.9 &  80 &  0.89 &   0.99 &     0.99 &     6.88 &          0.82 &              10.18 &                8.36 &  316.346 \\
 12 AM - 3 AM &   after &    1.0 &  20 &  0.89 &   0.99 &     0.99 &     6.87 &          0.81 &               4.92 &                6.21 &  86.2964 \\
 12 AM - 3 AM &   after &    1.0 &  40 &  0.89 &   0.99 &     0.99 &     6.89 &          0.82 &              11.01 &                8.70 &  169.562 \\
 12 AM - 3 AM &   after &    1.0 &  60 &  0.89 &   0.99 &     0.99 &     6.89 &          0.82 &              13.45 &                9.70 &  255.515 \\
 12 AM - 3 AM &   after &    1.0 &  80 &  0.89 &   0.99 &     0.99 &     6.89 &          0.82 &              15.15 &               10.40 &  342.193 \\
 12 AM - 3 AM &   after &    1.1 &  20 &  0.89 &   0.99 &     0.99 &     6.88 &          0.82 &              11.03 &                8.71 &  92.9921 \\
 12 AM - 3 AM &   after &    1.1 &  40 &  0.90 &   0.99 &     0.99 &     6.90 &          0.83 &              17.51 &               11.36 &  182.367 \\
 12 AM - 3 AM &   after &    1.1 &  60 &  0.89 &   0.99 &     0.99 &     6.91 &          0.83 &              20.06 &               12.40 &  274.834 \\
 12 AM - 3 AM &   after &    1.1 &  80 &  0.90 &   0.99 &     0.99 &     6.91 &          0.83 &              22.14 &               13.25 &  368.361 \\
 12 AM - 3 AM &   after &    1.2 &  20 &  0.90 &   0.99 &     0.99 &     6.90 &          0.82 &              15.82 &               10.67 &  98.9409 \\
 12 AM - 3 AM &   after &    1.2 &  40 &  0.90 &   0.99 &     0.99 &     6.91 &          0.83 &              22.89 &               13.56 &  196.371 \\
 12 AM - 3 AM &   after &    1.2 &  60 &  0.90 &   0.99 &     0.99 &     6.92 &          0.83 &              26.46 &               15.02 &  295.777 \\
 12 AM - 3 AM &   after &    1.2 &  80 &  0.90 &   0.99 &     0.99 &     6.93 &          0.83 &              28.82 &               15.98 &  393.446 \\
\bottomrule
\end{tabular}
\end{table}

\subsection{Detailed results for Algorithm~\ref{algo:greedy_algo}}

\begin{table}[H]
    \centering
    \scriptsize
    \caption{Results of the rule-based algorithm and comparison with historical trajectory}
    \label{tab:rerouting_performance_comparison_algo2}
    \begin{tabular}{c|c|c|c|c|c|c|c|c|c|c|c}
    \toprule
    $t$                       & Scenario               &$\delta$ & $K$& $c^{exp}$& $c^{inf}$ & $c^{imp}$ &  $H^{t}$  & $S^{t}$ & $\Delta D$& $\Delta T$ & CPU\_Time\\\hline
 9 AM - 12 PM &  before &    - &  - &  0.733 &  0.962 &    0.967 &    6.434 &         0.567 &               0.00 &                0.00 &     - \\
 9 AM - 12 PM &   after &    0.9 &  1 &  0.803 &  0.978 &    0.977 &    6.441 &         0.621 &             -19.69 &               46.10 &       2.0 \\
 9 AM - 12 PM &   after &    1.0 &  1 &  0.805 &  0.978 &    0.977 &    6.445 &         0.623 &             -19.16 &               46.15 &       2.0 \\
 9 AM - 12 PM &   after &    1.1 &  1 &  0.823 &  0.981 &    0.979 &    6.456 &         0.631 &             -14.33 &               45.96 &       2.0 \\
 9 AM - 12 PM &   after &    1.2 &  1 &  0.829 &  0.983 &    0.981 &    6.463 &         0.636 &             -10.08 &               45.50 &       2.0 \\\hline
 12 PM - 3 PM &  before &    - &  - &  0.760 &  0.976 &    0.977 &    6.594 &         0.629 &               0.00 &                0.00 &     - \\
  12 PM - 3 PM &   after &    0.9 &  1 &  0.843 &  0.989 &    0.985 &    6.611 &         0.686 &             -11.69 &               54.01 &       2.4 \\
 12 PM - 3 PM &   after &    1.0 &  1 &  0.850 &  0.989 &    0.985 &    6.616 &         0.690 &              -9.47 &               54.20 &       2.4 \\
 12 PM - 3 PM &   after &    1.1 &  1 &  0.856 &  0.989 &    0.985 &    6.619 &         0.694 &              -7.12 &               54.13 &       2.4 \\
 12 PM - 3 PM &   after &    1.2 &  1 &  0.858 &  0.989 &    0.985 &    6.621 &         0.695 &              -6.45 &               54.04 &       2.4 \\\hline
  3 PM - 6 PM &  before &    - &  - &  0.755 &  0.972 &    0.973 &    6.504 &         0.612 &               0.00 &                0.00 &     - \\
   3 PM - 6 PM &   after &    0.9 &  1 &  0.842 &  0.985 &    0.983 &    6.526 &         0.668 &             -10.22 &               54.11 &       2.4 \\
  3 PM - 6 PM &   after &    1.0 &  1 &  0.844 &  0.986 &    0.983 &    6.528 &         0.670 &             -10.01 &               54.65 &       2.4 \\
  3 PM - 6 PM &   after &    1.1 &  1 &  0.848 &  0.986 &    0.983 &    6.531 &         0.673 &              -8.47 &               54.68 &       2.3 \\
  3 PM - 6 PM &   after &    1.2 &  1 &  0.851 &  0.986 &    0.983 &    6.534 &         0.675 &              -5.75 &               54.71 &       2.4 \\\hline
  6 PM - 9 PM &  before &    - &  - &  0.761 &  0.974 &    0.975 &    6.561 &         0.622 &               0.00 &                0.00 &     - \\
    6 PM - 9 PM &   after &    0.9 &  1 &  0.824 &  0.983 &    0.981 &    6.589 &         0.668 &              -8.98 &               49.95 &       2.5 \\
  6 PM - 9 PM &   after &    1.0 &  1 &  0.832 &  0.985 &    0.982 &    6.594 &         0.673 &              -6.42 &               50.35 &       2.5 \\
  6 PM - 9 PM &   after &    1.1 &  1 &  0.834 &  0.985 &    0.982 &    6.597 &         0.676 &              -3.56 &               50.43 &       2.5 \\
  6 PM - 9 PM &   after &    1.2 &  1 &  0.837 &  0.985 &    0.982 &    6.599 &         0.677 &              -1.92 &               50.51 &       2.5 \\\hline
 9 PM - 12 AM &  before &    - &  - &  0.755 &  0.974 &    0.975 &    6.487 &         0.640 &               0.00 &                0.00 &     - \\
   9 PM - 12 AM &   after &    0.9 &  1 &  0.843 &  0.985 &    0.982 &    6.565 &         0.713 &             -16.11 &               54.32 &       3.5 \\
 9 PM - 12 AM &   after &    1.0 &  1 &  0.848 &  0.985 &    0.982 &    6.569 &         0.716 &             -15.59 &               54.41 &       3.6 \\
 9 PM - 12 AM &   after &    1.1 &  1 &  0.849 &  0.985 &    0.982 &    6.572 &         0.718 &             -14.72 &               54.39 &       3.6 \\
 9 PM - 12 AM &   after &    1.2 &  1 &  0.857 &  0.987 &    0.984 &    6.579 &         0.723 &             -12.40 &               54.12 &       3.6 \\\hline
 12 AM - 3 AM &  before &    - &  - &  0.773 &  0.976 &    0.976 &    6.586 &         0.666 &               0.00 &                0.00 &     - \\
 12 AM - 3 AM &   after &    0.9 &  1 &  0.853 &  0.991 &    0.988 &    6.644 &         0.738 &             -12.97 &               50.10 &       4.1 \\
 12 AM - 3 AM &   after &    1.0 &  1 &  0.856 &  0.991 &    0.988 &    6.648 &         0.741 &             -12.22 &               50.23 &       4.0 \\
 12 AM - 3 AM &   after &    1.1 &  1 &  0.862 &  0.991 &    0.988 &    6.654 &         0.745 &             -10.23 &               50.07 &       4.1 \\
 12 AM - 3 AM &   after &    1.2 &  1 &  0.864 &  0.991 &    0.988 &    6.658 &         0.748 &              -8.61 &               49.83 &       4.1 \\
\bottomrule
\end{tabular}
\end{table}
